# Supplementary material for: Transparent IFC Enforcement: Possibility and (In)Efficiency Results
Source: arXiv:2005.12345 source file (2020-05-25)
Supplement: Supplementary file 1 [file encoding-appendix.tex]

Readers who are accustomed to a different framework or semantic model
may find it useful to consider how this framework maps onto existing
models of secure computation in the literature.
We claim that our formulation is natural, to demonstrate this we
construct mappings to a number of notions from the literature on
information flow control.
The goal is to show that for a given notion of computation, where
programs are on the form $p : T_i \pto T_o$ we can provide
$A$ and $B$ as well as functions $\inputify : \Pow{A \times \L} \to T_i$ and
$\outputify : T_o \to \Pow{B \times \L}$.
Naturally, $\inputify$ and $\outputify$ have certain correctness criteria associated
with them.
Among other things, $\inputify$ needs to be onto and $\outputify$ one-to-one.
However, we omit a fully formal development of this requirements in the
interest of brevity.

We begin by establishing the connection between this model and the use of statically
labeled input and output channels.
\begin{example}[Static Channels]
  \label{ex:static-encoding}
  Devriese and Piessens \cite{SME} present a program calculus with statically labeled
  input and output channels.
  Under their system, a program $p$ has associated with it a set of input channels $I_p$
  and a set of output channels $O_p$.
  Each input channel $i \in I_p$ has an associated level $\ell_i$ and each output channel
  $o \in O_p$ an associated level $\jmath_o$.
  For simplicity, we consider the case where each channel carries one natural number.
  This means that a program $p$ is a partial function $p : (I_p \to \Nat) \pto (O_p \to \Nat)$

  Next we need to adapt programs on this form to our setting.
  We choose the domain to be $I_p \times \Nat$ and the co-domain to be $O_p \times \Nat$.
  From a set $x \in \Pow{(I_p \times \Nat) \times \L}$ we can construct a map $x' : (I_p \to \Nat)$
  to correspond to the input of $p$ by constructing, for example:
  $$
  \inputify(x) = \lambda i.\ |x@\ell_i|
  $$
  We could, of course, have chosen $\inputify(x) = \lambda i.\ \Sigma_{(i, v, \ell_i) \in x@\ell_i} v$.
  The point of this is to illustrate that sets of values are a sufficiently
  expressive notion to allow us to capture many different semantics.

  From the \emph{finite} output map $y : O_p \to \Nat$ we need to construct a set
  in $\Pow{(O_p \times \Nat) \times \L}$, this is trivial to do:
  $$
  \outputify(y) = \{ (o, y(o))^{\jmath_o}\ |\ o \in \text{domain}(y)\ \}
  $$
  Finally, we can construct the program $q : \Pow{(I_p \times \Nat) \times \L} \pto \Pow{(O_p \times \Nat) \times \L}$
  as:
  $$
  \sem{q}(x) = \outputify(\sem{p}(\inputify(x)))
  $$

  One point of departure in this presentation from that of Devriese and Piessens is that
  they are in a reactive setting.
  Therefore, they consider channels with streams of input and output.
  We discuss extending the results of this paper to the reactive setting in Section \ref{sec:future-work}.
\end{example}
Next we consider a dynamic model of secure computation, where labels are not necessarily known
a-priori.
\begin{example}[Flow Sensitive Labels]
  Kozyri et al. \cite{kozyri2019beyond}, Hritcu et al. \cite{hritcu2013all}, and others have
  presented program calculi with \emph{flow-sensitive} dynamic labels.
  In these systems, program variables and outputs have associated labels that change
  during program execution.
  Crucially, the labels on the final program outputs can be decided dynamically.

  We assume, in the interest of simplicity, that the label on each program input 
  is decided \emph{a priori} by a public function $L : \text{Var} \to \L$.
  In this simplified setting, we assign the type
  $$(\text{Var} \to \Nat) \to ((\text{Var} \to \Nat) \times (\text{Var} \to \L))$$
  to their programs.
  Technically, the papers mentioned above consider also labels-on-labels, and
  labels-on-labels-on-labels etc.
  While such constructions can be encoded in our framework, we choose to keep
  things simple here.
  We pick both the domain ($A$) and co-domain ($B$) to be $\text{Var} \times \Nat$.
  Constructing the $\inputify$ function is trivial:
  $$
  \inputify(x) = \lambda v.\ |\{ i\ |\ (v, i)^\ell \in x@L(v) \}|
  $$
  Next we need to construct a version of $\outputify$ for dynamically labeled outputs.
  $$
  \outputify((\nu,\ell)) = \{(v, \nu(i))^{\ell(v)}\ |\ v \in \text{domain}(\nu) \}
  $$
\end{example}
Finally, we consider the model of \emph{Multiple Facets} (MF), a model used both for
enforcing noninterference transparently \cite{MF}, as well as a programming model to
aide secure development \cite{yang2016precise}.
\begin{example}[Multiple Facets]
  Austin and Flanagan introduce Multiple Facets (MF) \cite{MF}, a program semantics whereby
  each program variable $x$ corresponds to a function $x : \L \to \text{Value}$.
  Under their scheme, a program is a partial recursive function
  $p : (\text{Var} \to \L \to \Nat) \pto (\text{Var} \to \L \to \Nat)$.
  We can model this by picking the domain and co-domain to be $\text{Var} \times \Nat$.
  Where we have an analogous definition of $\inputify$ to the case for static channels:
  $$
  \inputify(x) = \lambda v.\ \lambda \ell.\ |\{ i\ |\ (v, i)^\ell \in x@\ell\}|
  $$
  And for $\outputify$ we do something similar to the above cases:
  $$
  \outputify(f) = \{ (v, f(v, \ell))^\ell\ |\ (v, \ell) \in \text{domain}(f) \}
  $$
\end{example}
